# Supplementary material for: Enhancing Tabular Reasoning with Pattern Exploiting Training
Source: arXiv:2210.12259 source file (2022-10-21)
Supplement: Supplementary file 1 [file appendix_latex.tex]

% % This must be in the first 5 lines to tell arXiv to use pdfLaTeX, which is strongly recommended.
% \pdfoutput=1
% % In particular, the hyperref package requires pdfLaTeX in order to break URLs across lines.

% \documentclass[11pt]{article}

% % Remove the "review" option to generate the final version.
% \usepackage[review]{acl}
% % \usepackage{acl}

% % Standard package includes
% \usepackage{times}
% \usepackage{latexsym}

% % For proper rendering and hyphenation of words containing Latin characters (including in bib files)
% \usepackage[T1]{fontenc}
% % For Vietnamese characters
% % \usepackage[T5]{fontenc}
% % See https://www.latex-project.org/help/documentation/encguide.pdf for other character sets

% % This assumes your files are encoded as UTF8
% \usepackage[utf8]{inputenc}

% % This is not strictly necessary, and may be commented out,
% % but it will improve the layout of the manuscript,
% % and will typically save some space.
% % \usepackage{bigfoot}
% % \usepackage[bottom]{footmisc} 
% \usepackage{amsmath,array,graphicx}
% \usepackage{lipsum}
% \usepackage{cleveref}
% \crefname{section}{§}{§§}
% \usepackage{microtype}
% \usepackage{tabularx}
% \usepackage{multirow}
% \usepackage{booktabs}
% \usepackage{arydshln}
% \definecolor{cadmiumgreen}{rgb}{0.0, 0.42, 0.24}
% \usepackage{paralist}
% \usepackage[para]{footmisc}
% \usepackage{natbib}
% \usepackage{xspace}
% \usepackage{adjustbox}
% \usepackage{tikzit}
% \input{sample.tikzstyles}
% % \usepackage{xurl}
% % \usepackage[para]{footmisc}
% % If the title and author information does not fit in the area allocated, uncomment the following
% %
% %\setlength\titlebox{<dim>}
% %
% % and set <dim> to something 5cm or larger.

% \title{Enhancing Tabular Reasoning with Pattern Exploiting Training\\Appendix}

% % Author information can be set in various styles:
% % For several authors from the same institution:
% % \author{Author 1 \and ... \and Author n \\
% %         Address line \\ ... \\ Address line}
% % if the names do not fit well on one line use
% %         Author 1 \\ {\bf Author 2} \\ ... \\ {\bf Author n} \\
% % For authors from different institutions:
% % \author{Author 1 \\ Address line \\  ... \\ Address line
% %         \And  ... \And
% %         Author n \\ Address line \\ ... \\ Address line}
% % To start a seperate ``row'' of authors use \AND, as in
% % \author{Author 1 \\ Address line \\  ... \\ Address line
% %         \AND
% %         Author 2 \\ Address line \\ ... \\ Address line \And
% %         Author 3 \\ Address line \\ ... \\ Address line}

% \author {
%     % Authors
%     Abhilash Shankarampeta\textsuperscript{\rm 1\thanks{ Equal Contribution}},
%     Vivek Gupta\textsuperscript{\rm {2*}\thanks{ Corresponding Author}}
%     \\\textsuperscript{\rm 1}IIT Guwahati;
%      \textsuperscript{\rm 2}University of Utah\\
%     sareddy53@gmail.com; vgupta@cs.utah.edu;
% }

% \newcommand{\datasetName}{{\sc InfoTabS}\xspace}
% \newcommand{\alphaOne}{$\alpha_1$\xspace}
% \newcommand{\alphaTwo}{$\alpha_2$\xspace}
% \newcommand{\alphaThree}{$\alpha_3$\xspace}


% \newcommand{\vg}[1]{[\textcolor{red}{$^V_G$ \small  #1}]} 
% \newcommand{\as}[1]{[\textcolor{purple}{$^a_s$ \small #1}]}
% \newcommand{\sz}[1]{[\textcolor{blue}{$^s_z$ \small #1}]}

% \begin{document}
% \maketitle
% % \begin{abstract}
% % Recent methods based on pre-trained language models have exhibited superior performance when reasoning over tabular data, despite showing inherent problems  with reasoning over tabular data \citep{gupta2021my}. In this work, we utilize Pattern-Exploiting Training (PET) to strengthen pre-existing knowledge and reasoning abilities of these tabular reasoning models'. In comparison to current baselines, our upgraded model exhibits superior understanding of knowledge facts and tabular reasoning. Additionally, we demonstrate that such models are more effective for underlying downstream task of tabular inference on InfoTabS. Furthermore, we also shows our model's robustness against adversarial sets generated through various character and word level perturbations on InfoTabS testset.

% % Recent methods based on pre-trained language models have exhibited superior performance over tabular tasks (e.g., tabular NLI), despite showing inherent problems such as not using the right evidence, inconsistent predictions across inputs while reasoning over the tabular data \citep{DBLP:journals/corr/abs-2108-00578}. In this work, we utilize Pattern-Exploiting Training (PET) (i.e., strategic MLM) on pre-trained language models to strengthen these tabular reasoning models' pre-existing knowledge and reasoning abilities. Our upgraded model exhibits a superior understanding of knowledge facts and tabular reasoning compared to current baselines. Additionally, we demonstrate that such models are more effective for underlying downstream tasks of tabular inference on \datasetName~. Furthermore, we show our model's robustness against adversarial sets generated through various character and word level perturbations.

% % \end{abstract}

% % The existing factual and relational knowledge of these models about the data has deteriorated significantly.
% % \section{Introduction}

% % These instructions are for authors submitting papers to *ACL conferences using \LaTeX. They are not self-contained. All authors must follow the general instructions for *ACL proceedings,\footnote{\url{http://acl-org.github.io/ACLPUB/formatting.html}} and this document contains additional instructions for the \LaTeX{} style files.

% % The templates include the \LaTeX{} source of this document (\texttt{acl.tex}),
% % the \LaTeX{} style file used to format it (\texttt{acl.sty}),
% % an ACL bibliography style (\texttt{acl\_natbib.bst}),
% % an example bibliography (\texttt{custom.bib}),
% % and the bibliography for the ACL Anthology (\texttt{anthology.bib}).

% % \input{Sections/intro}
% % \input{Sections/motive}
% % \input{Sections/method}
% % \input{Sections/experiments}
% % \input{Sections/Discussion}
% % \input{Sections/RelatedWork}
% % \input{Sections/Conclusion}
% % % \input{Sections/Acknowledgement}
% % \input{Sections/limitation}
% % \input{Sections/table}
% % \section{Experiments and Analysis}

% % % To produce a PDF file, pdf\LaTeX{} is strongly recommended (over original \LaTeX{} plus dvisps+ps2pdf or dvipdf). Xe\LaTeX{} also produces PDF files, and is especially suitable for text in non-Latin scripts.

% % \section{Preamble}

% % The first line of the file must be
% % \begin{quote}
% % \begin{verbatim}
% % \documentclass[11pt]{article}
% % \end{verbatim}
% % \end{quote}

% % To load the style file in the review version:
% % \begin{quote}
% % \begin{verbatim}
% % \usepackage[review]{acl}
% % \end{verbatim}
% % \end{quote}
% % For the final version, omit the \verb|review| option:
% % \begin{quote}
% % \begin{verbatim}
% % \usepackage{acl}
% % \end{verbatim}
% % \end{quote}

% % To use Times Roman, put the following in the preamble:
% % \begin{quote}
% % \begin{verbatim}
% % \usepackage{times}
% % \end{verbatim}
% % \end{quote}
% % (Alternatives like txfonts or newtx are also acceptable.)

% % Please see the \LaTeX{} source of this document for comments on other packages that may be useful.

% % Set the title and author using \verb|\title| and \verb|\author|. Within the author list, format multiple authors using \verb|\and| and \verb|\And| and \verb|\AND|; please see the \LaTeX{} source for examples.

% % By default, the box containing the title and author names is set to the minimum of 5 cm. If you need more space, include the following in the preamble:
% % \begin{quote}
% % \begin{verbatim}
% % \setlength\titlebox{<dim>}
% % \end{verbatim}
% % \end{quote}
% % where \verb|<dim>| is replaced with a length. Do not set this length smaller than 5 cm.

% % \section{Document Body}

% % \subsection{Footnotes}

% % Footnotes are inserted with the \verb|\footnote| command.\footnote{This is a footnote.}

% % \subsection{Tables and figures}

% % See Table~\ref{tab:accents} for an example of a table and its caption.
% % \textbf{Do not override the default caption sizes.}

% % \begin{table}
% % \centering
% % \begin{tabular}{lc}
% % \hline
% % \textbf{Command} & \textbf{Output}\\
% % \hline
% % \verb|{\"a}| & {\"a} \\
% % \verb|{\^e}| & {\^e} \\
% % \verb|{\`i}| & {\`i} \\ 
% % \verb|{\.I}| & {\.I} \\ 
% % \verb|{\o}| & {\o} \\
% % \verb|{\'u}| & {\'u}  \\ 
% % \verb|{\aa}| & {\aa}  \\\hline
% % \end{tabular}
% % \begin{tabular}{lc}
% % \hline
% % \textbf{Command} & \textbf{Output}\\
% % \hline
% % \verb|{\c c}| & {\c c} \\ 
% % \verb|{\u g}| & {\u g} \\ 
% % \verb|{\l}| & {\l} \\ 
% % \verb|{\~n}| & {\~n} \\ 
% % \verb|{\H o}| & {\H o} \\ 
% % \verb|{\v r}| & {\v r} \\ 
% % \verb|{\ss}| & {\ss} \\
% % \hline
% % \end{tabular}
% % \caption{Example commands for accented characters, to be used in, \emph{e.g.}, Bib\TeX{} entries.}
% % \label{tab:accents}
% % \end{table}

% % \subsection{Hyperlinks}

% % Users of older versions of \LaTeX{} may encounter the following error during compilation: 
% % \begin{quote}
% % \tt\verb|\pdfendlink| ended up in different nesting level than \verb|\pdfstartlink|.
% % \end{quote}
% % This happens when pdf\LaTeX{} is used and a citation splits across a page boundary. The best way to fix this is to upgrade \LaTeX{} to 2018-12-01 or later.

% % \subsection{Citations}

% % \begin{table*}
% % \centering
% % \begin{tabular}{lll}
% % \hline
% % \textbf{Output} & \textbf{natbib command} & \textbf{Old ACL-style command}\\
% % \hline
% % \citep{Gusfield:97} & \verb|\citep| & \verb|\cite| \\
% % \citealp{Gusfield:97} & \verb|\citealp| & no equivalent \\
% % \citet{Gusfield:97} & \verb|\citet| & \verb|\newcite| \\
% % \citeyearpar{Gusfield:97} & \verb|\citeyearpar| & \verb|\shortcite| \\
% % \hline
% % \end{tabular}
% % \caption{\label{citation-guide}
% % Citation commands supported by the style file.
% % The style is based on the natbib package and supports all natbib citation commands.
% % It also supports commands defined in previous ACL style files for compatibility.
% % }
% % \end{table*}

% % Table~\ref{citation-guide} shows the syntax supported by the style files.
% % We encourage you to use the natbib styles.
% % You can use the command \verb|\citet| (cite in text) to get ``author (year)'' citations, like this citation to a paper by \citet{Gusfield:97}.
% % You can use the command \verb|\citep| (cite in parentheses) to get ``(author, year)'' citations \citep{Gusfield:97}.
% % You can use the command \verb|\citealp| (alternative cite without parentheses) to get ``author, year'' citations, which is useful for using citations within parentheses (e.g. \citealp{Gusfield:97}).

% % \subsection{References}

% % \nocite{Ando2005,borschinger-johnson-2011-particle,andrew2007scalable,rasooli-tetrault-2015,goodman-etal-2016-noise,harper-2014-learning}

% % The \LaTeX{} and Bib\TeX{} style files provided roughly follow the American Psychological Association format.
% % If your own bib file is named \texttt{custom.bib}, then placing the following before any appendices in your \LaTeX{} file will generate the references section for you:
% % \begin{quote}
% % \begin{verbatim}
% % \bibliographystyle{acl_natbib}
% % \bibliography{custom}
% % \end{verbatim}
% % \end{quote}

% % You can obtain the complete ACL Anthology as a Bib\TeX{} file from \url{https://aclweb.org/anthology/anthology.bib.gz}.
% % To include both the Anthology and your own .bib file, use the following instead of the above.
% % \begin{quote}
% % \begin{verbatim}
% % \bibliographystyle{acl_natbib}
% % \bibliography{anthology,custom}
% % \end{verbatim}
% % \end{quote}

% % Please see Section~\ref{sec:bibtex} for information on preparing Bib\TeX{} files.

% % \subsection{Appendices}

% % Use \verb|\appendix| before any appendix section to switch the section numbering over to letters. See Appendix~\ref{sec:appendix} for an example.

% % \section{Bib\TeX{} Files}
% % \label{sec:bibtex}

% % Unicode cannot be used in Bib\TeX{} entries, and some ways of typing special characters can disrupt Bib\TeX's alphabetization. The recommended way of typing special characters is shown in Table~\ref{tab:accents}.

% % Please ensure that Bib\TeX{} records contain DOIs or URLs when possible, and for all the ACL materials that you reference.
% % Use the \verb|doi| field for DOIs and the \verb|url| field for URLs.
% % If a Bib\TeX{} entry has a URL or DOI field, the paper title in the references section will appear as a hyperlink to the paper, using the hyperref \LaTeX{} package.

% % \section*{Acknowledgements}

% % This document has been adapted
% % by Steven Bethard, Ryan Cotterell and Rui Yan
% % from the instructions for earlier ACL and NAACL proceedings, including those for 
% % ACL 2019 by Douwe Kiela and Ivan Vuli\'{c},
% % NAACL 2019 by Stephanie Lukin and Alla Roskovskaya, 
% % ACL 2018 by Shay Cohen, Kevin Gimpel, and Wei Lu, 
% % NAACL 2018 by Margaret Mitchell and Stephanie Lukin,
% % Bib\TeX{} suggestions for (NA)ACL 2017/2018 from Jason Eisner,
% % ACL 2017 by Dan Gildea and Min-Yen Kan, 
% % NAACL 2017 by Margaret Mitchell, 
% % ACL 2012 by Maggie Li and Michael White, 
% % ACL 2010 by Jing-Shin Chang and Philipp Koehn, 
% % ACL 2008 by Johanna D. Moore, Simone Teufel, James Allan, and Sadaoki Furui, 
% % ACL 2005 by Hwee Tou Ng and Kemal Oflazer, 
% % ACL 2002 by Eugene Charniak and Dekang Lin, 
% % and earlier ACL and EACL formats written by several people, including
% % John Chen, Henry S. Thompson and Donald Walker.
% % Additional elements were taken from the formatting instructions of the \emph{International Joint Conference on Artificial Intelligence} and the \emph{Conference on Computer Vision and Pattern Recognition}.

% \appendix
% \input{Sections/appendix}
% % \newpage
% \input{Sections/limitation}

% % Entries for the entire Anthology, followed by custom entries
% \bibliography{anthology,custom}
% \bibliographystyle{acl_natbib}



% % \section{Appendix}
% % \label{sec:appendix}


% % This is an appendix.

% \end{document}
